# Supplementary material for: Valve: Production Online-Offline Inference Colocation with Jointly-Bounded Preemption Latency and Rate
Source: arXiv:2604.07874 source file (2026-04-09)
Supplement: Supplementary file 1 [file appendix.tex]

\appendix
\section{Appendix}

\subsection{Optimality of Algorithm~\ref{alg:design:opt-process}}
\label{apdx:opt-process}

\begin{theorem}\label{theorem:opt-process}
    Algorithm~\ref{alg:design:opt-process} finds the optimal range configuration that minimizes the normalized 
    iteration latency.
\end{theorem}
